# Supplementary material for: Saturn: An Optimized Data System for Large Model Deep Learning Workloads
Source: arXiv:2309.01226 source file (2023-12-13)
Supplement: Supplementary file 1 [file appendix.tex]

%\vspace{-2mm}
\appendix
\section{\system~API Usage Example}\label{sec:appendix_api}
In this section, we provide detailed pseudocode illustrating examples of: (1) registering a new UPP with \system, (2) invoking the profiler, and (3) calling the executor.

\textbf{UPP Registration \& Specification}
As discussed in Section~\ref{sec:workload_spec}, the user can specify a UPP by implementing two functions --- one for knob-tuning, and one for execution.
Listing~\ref{lst:parallelism_spec} provides condensed pseudocode demonstrating how to register Fully Sharded Data Parallelism (provided in the PyTorch Distributed package) with \system.
The full code is available at our GitHub repository.

\begin{lstlisting}[language=Python, label={lst:parallelism_spec},caption=Registering FSDP as a UPP in \system's Library.,frame=single]
class FSDPExecutor(BaseTechnique):

	def execute(task, gpus):
		WORLD_SIZE = len(gpus)
		
		def distributed_function(rank, world_size, task, gpus):
			setup()
			model, loss_fn = task.get_model(), task.loss_function
			knobs = task.strategy.knobs
			hints = task.hints
			
			if hints.is_transformer:
				wrap_policy = "transformer"
			else:
				wrap_policy = "auto"
			
			model = FSDP(model, offload=knobs.offload, device=rank, auto_wrap_policy=wrap_policy)
			if knobs.checkpoint:
				model = apply_checkpointing(model)
			
			lr = task.hparams.lr
			optimizer = task.hparams.optimizer_cls(model.parameters(), lr)
			
			execution_loop(model, task.iterator)
			

		multiprocessing.spawn(distributed_function, args=(task, gpus))
		
	def search(task, gpus):
		knob_search = [
			checkpoint: True, offload: True,
			checkpoint: True, offload: False,
			checkpoint: False, offload: True,
			checkpoint: False, offload: False
		]
		
		selected_config, runtime = None, None
		for config in knob_search:
			trial_task.knobs = config
			trial_task.length = 5 batches
			try:
				rt = time(execute(trial_task, gpus))
				if rt < runtime:
					selected_config = config
					runtime = rt
			except:
				continue
		
\end{lstlisting}

This class can now be registered with the parallelism library as illustrated in Listing~\ref{lst:technique_registration} in Section~\ref{sec:workload_spec}.
The newly added technique can now be automatically applied to newly submitted models for profiling \& execution.

\textbf{Profiling \& Execution}
The profiler allows us to estimate the performance of each model under different techniques with different GPU allocation levels.
Listing~\ref{lst:model_definition_and_profiling} illustrates an example of specifying, profiling, and executing two GPT-J fine-tuning jobs.
The base model is loaded from HuggingFace's model hub, before being passed into a Task wrapper with a hint for \system~to note that the model is a Transformer.

\begin{lstlisting}[language=Python, label={lst:model_definition_and_profiling},caption=Specifying a training job and launching it with \system.,frame=single]
from transformers.models.gptj import GPTJForCausalLM
from data import dataloaders

def load_model():
	configuration = GPTJConfig.from_pretrained("EleutherAI/gpt-j-6B", output_hidden_states=False)	
	model = GPTJForCausalLM.from_pretrained("EleutherAI/gpt-j-6B", config=configuration)	
	

hints = {transformer: True}
hparams_a = HParams(lr=1e-3, epochs=5, optimizer_cls=torch.optim.SGD)
hparams_b = HParams(lr=1e-5, epochs=5, optimizer_cls=torch.optim.Adam)
task_a = Task(load_model, dataloader, hints, hparams_a)
task_b = Task(load_model, dataloader, hints, hparams_b)


task_list = [task_a, task_b]
profile(task_list)
execute(task_list) # automatically invokes the MILP search procedure

\end{lstlisting}

\section{MILP Timeout Sensitivity}
One potential risk with our highly non-convex problem space is that the solver may get stuck in a local optimum. 
Given infinite time to optimize, an MILP solver may be able to guarantee that it will eventually reach the global optimum.
But we must enforce a more realistic timeout for practical purposes.
\system~sets a 5-minute timeout, and we generally find that this timeout is sufficient to produce a high-quality solution.
In this section, we empirically justify that choice of timeout by charting out achieved solution makespan against MILP solving time.
We demonstrate that increasing the timeout does not provide significant marginal improvements, implying that the 5-minute timeout already achieves a solution that compares favorably to the theoretical global optimum.

We reuse the single-node TXT simulation workload from Section~\ref{sec:milp_sim}. We do not consider introspection. The results are illustrated in Figure~\ref{fig:milp_scaling}.

\begin{figure}[H]
\includegraphics[width=0.95\columnwidth]{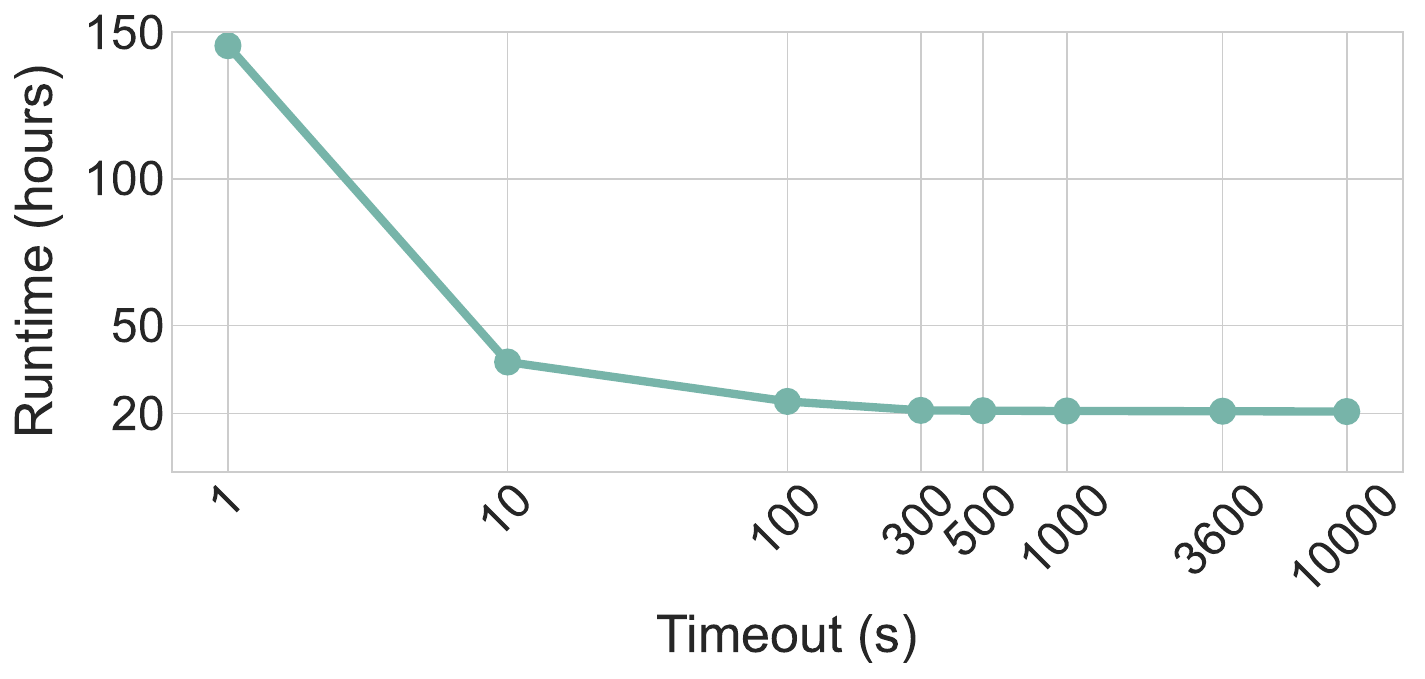}
\vspace{-3mm}
\caption{Achieved makespan on the single-node TXT workload as Gurobi's timeout is increased.}
\label{fig:milp_scaling}
\end{figure}

Past the 5-minute mark, the improvements are insubstantial. Going from a 5 minute timeout to a 1 hour timeout only reduces the achieved makespan by about 10 minutes (approx. $0.99\%$). 
It should be noted, however, that these results are specific to the tested workloads. Our end-to-end workloads are similar to this one in scale, and anecdotally, many model selection workloads are of a similar size.
Future iterations of \system~might look to automatically select a timeout depending on workload size. 
For example, a one-hundred model workload might require a longer optimization period, and correspondingly the higher overhead might be more tolerable in relation to the larger scale of the job.
For now, however, we simply expose the timeout to the user so that they can re-configure it if they feel that the default 5 minutes is not well-suited to the workload at hand.

\section{Illustrations of MILP Constraints}
In this section, we continue the illustration of our MILP constraints from Section~\ref{sec:milp}. Since Constraints 1-3 are already illustrated in the main text,
we will only illustrate Constraints 4-11 here.

\vspace{2mm}
\textbf{Constraints 4 and 5.}

Constraint 4 ensures that the total number of assigned GPUs (left hand-side of constraint) is $\geq$ the number of GPUs prescribed by the selected strategy.
Constraint 5 ensures a $\leq$ relationship between the two quantities. The combination of $\geq$ and $\leq$ yield a straightforward equality, which is not possible to formulate directly in an MILP.
So, we use this roundabout ``combination'' technique.

\vspace{-2mm}
\begin{align}
\tag{\ref{eqn:gpu_allocation_a}}
\begin{split}
\sum_{t \in P_{t,n}} t \geq G_{t,s} - U \times (2 - O_{t,n} - B_{t,s}) \forall s \in S_{t}, \forall t \in T, \forall n \in N
\end{split}
\end{align}

\vspace{-2mm}
\begin{align}
\tag{\ref{eqn:gpu_allocation_b}}
\begin{split}
\sum_{t \in P_{t,n}} t \leq G_{t,s} + U \times (2 - O_{t,n} - B_{t,s}) \forall s \in S_{t}, \forall t \in T, \forall n \in N
\end{split}
\end{align}

\begin{figure}[H]
\includegraphics[width=0.95\columnwidth]{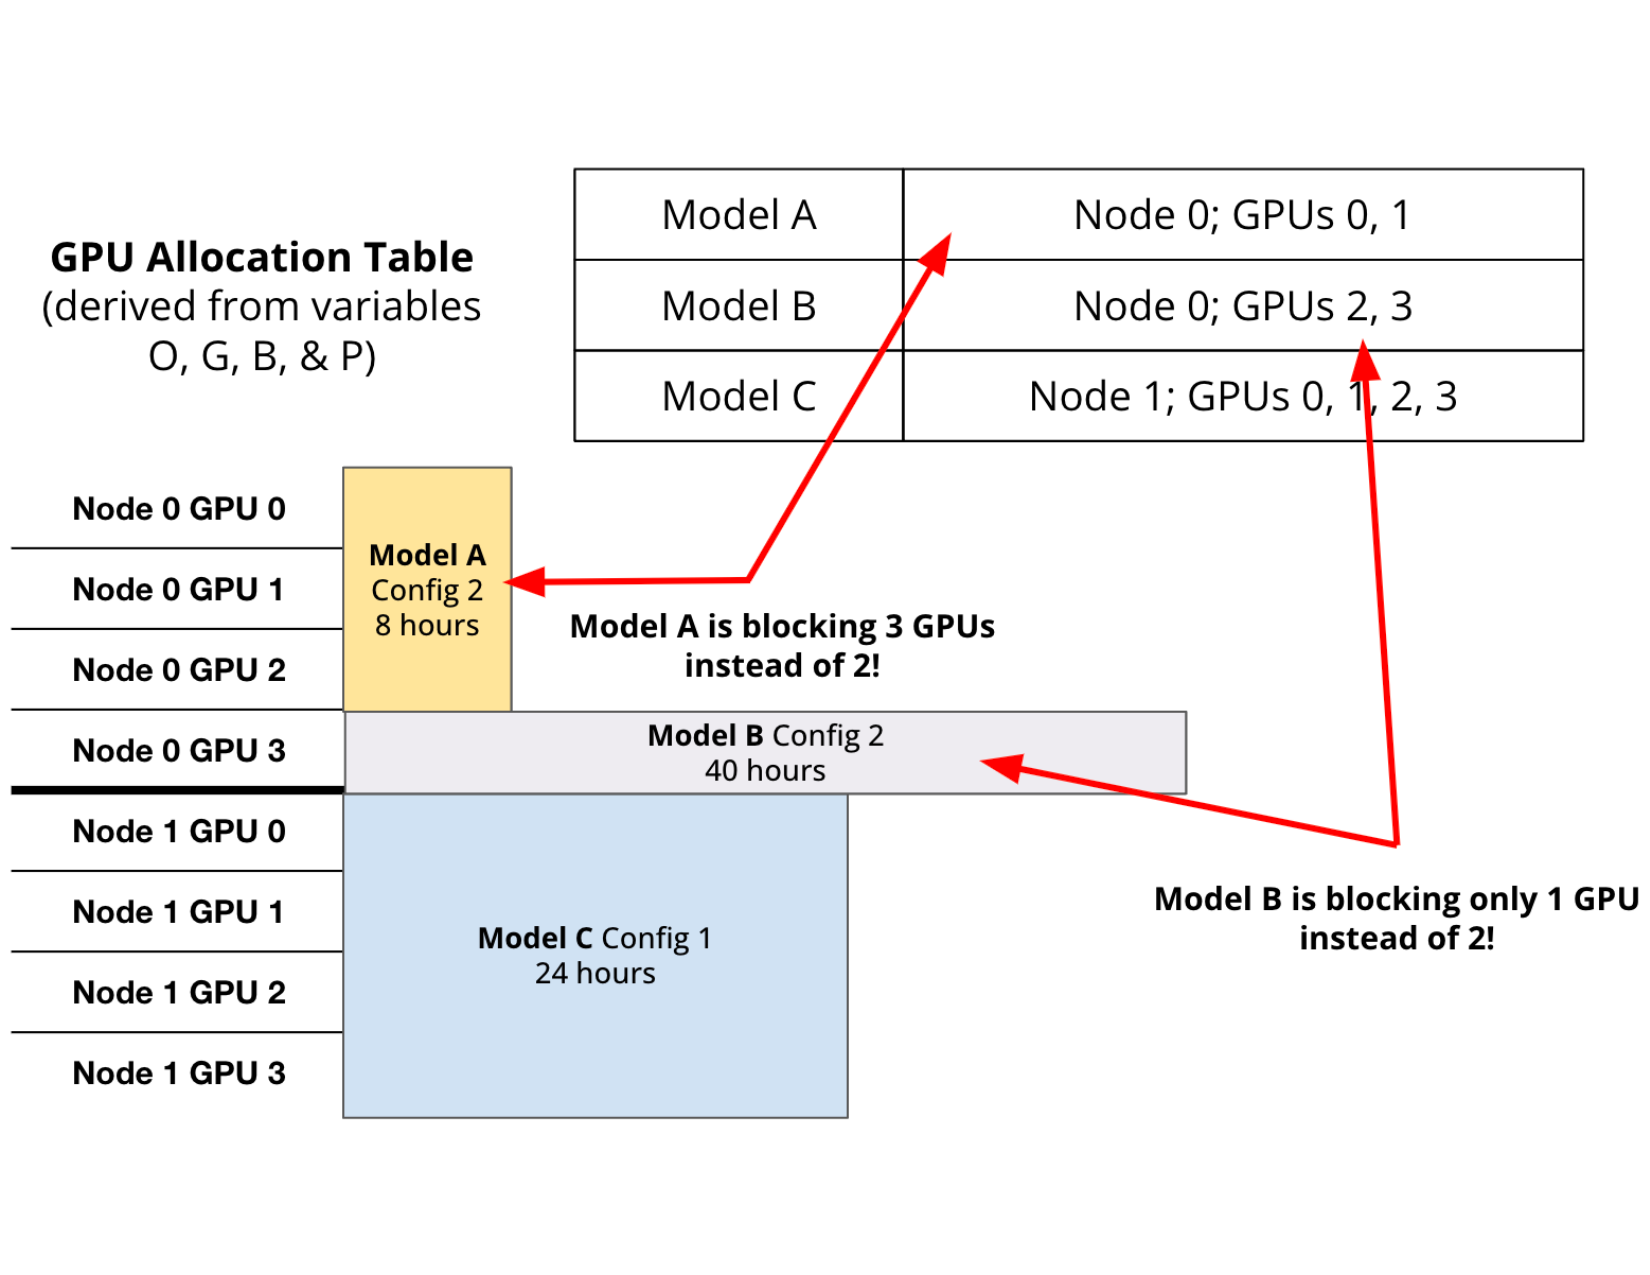}
\vspace{-3mm}
\caption{Illustration of a \spase~solution where tasks select too few or too many GPUs, violating constraints 4 \& 5.}
\label{fig:milp_illustration_constraint4}
\end{figure}

\vspace{2mm}

\textbf{Constraints 6 and 7.}

Constraints 6 \& 7 ensures that the total number of blocked GPUs on the node (left hand-side of constraint) is  0 if the node has not been selected.
We use the same combination procedure as in 4 \& 5.

\vspace{-2	mm}
\begin{align}
\tag{\ref{eqn:gpu_unallocation_a}}
\begin{split}
\sum_{t \in P_{t,n}} t~\red{\leq}~0 - U \times (O_{t,n} + B_{t,s}) \forall s \in S_{t}, \forall t \in T, \forall n \in N
\end{split}
\end{align}

\begin{align}
\tag{\ref{eqn:gpu_unallocation_b}}
\begin{split}
\sum_{t \in P_{t,n}} t~\red{\geq}~0 + U \times (O_{t,n} + B_{t,s}) \forall s \in S_{t}, \forall t \in T, \forall n \in N
\end{split}
\end{align}

\begin{figure}[H]
\includegraphics[width=0.95\columnwidth]{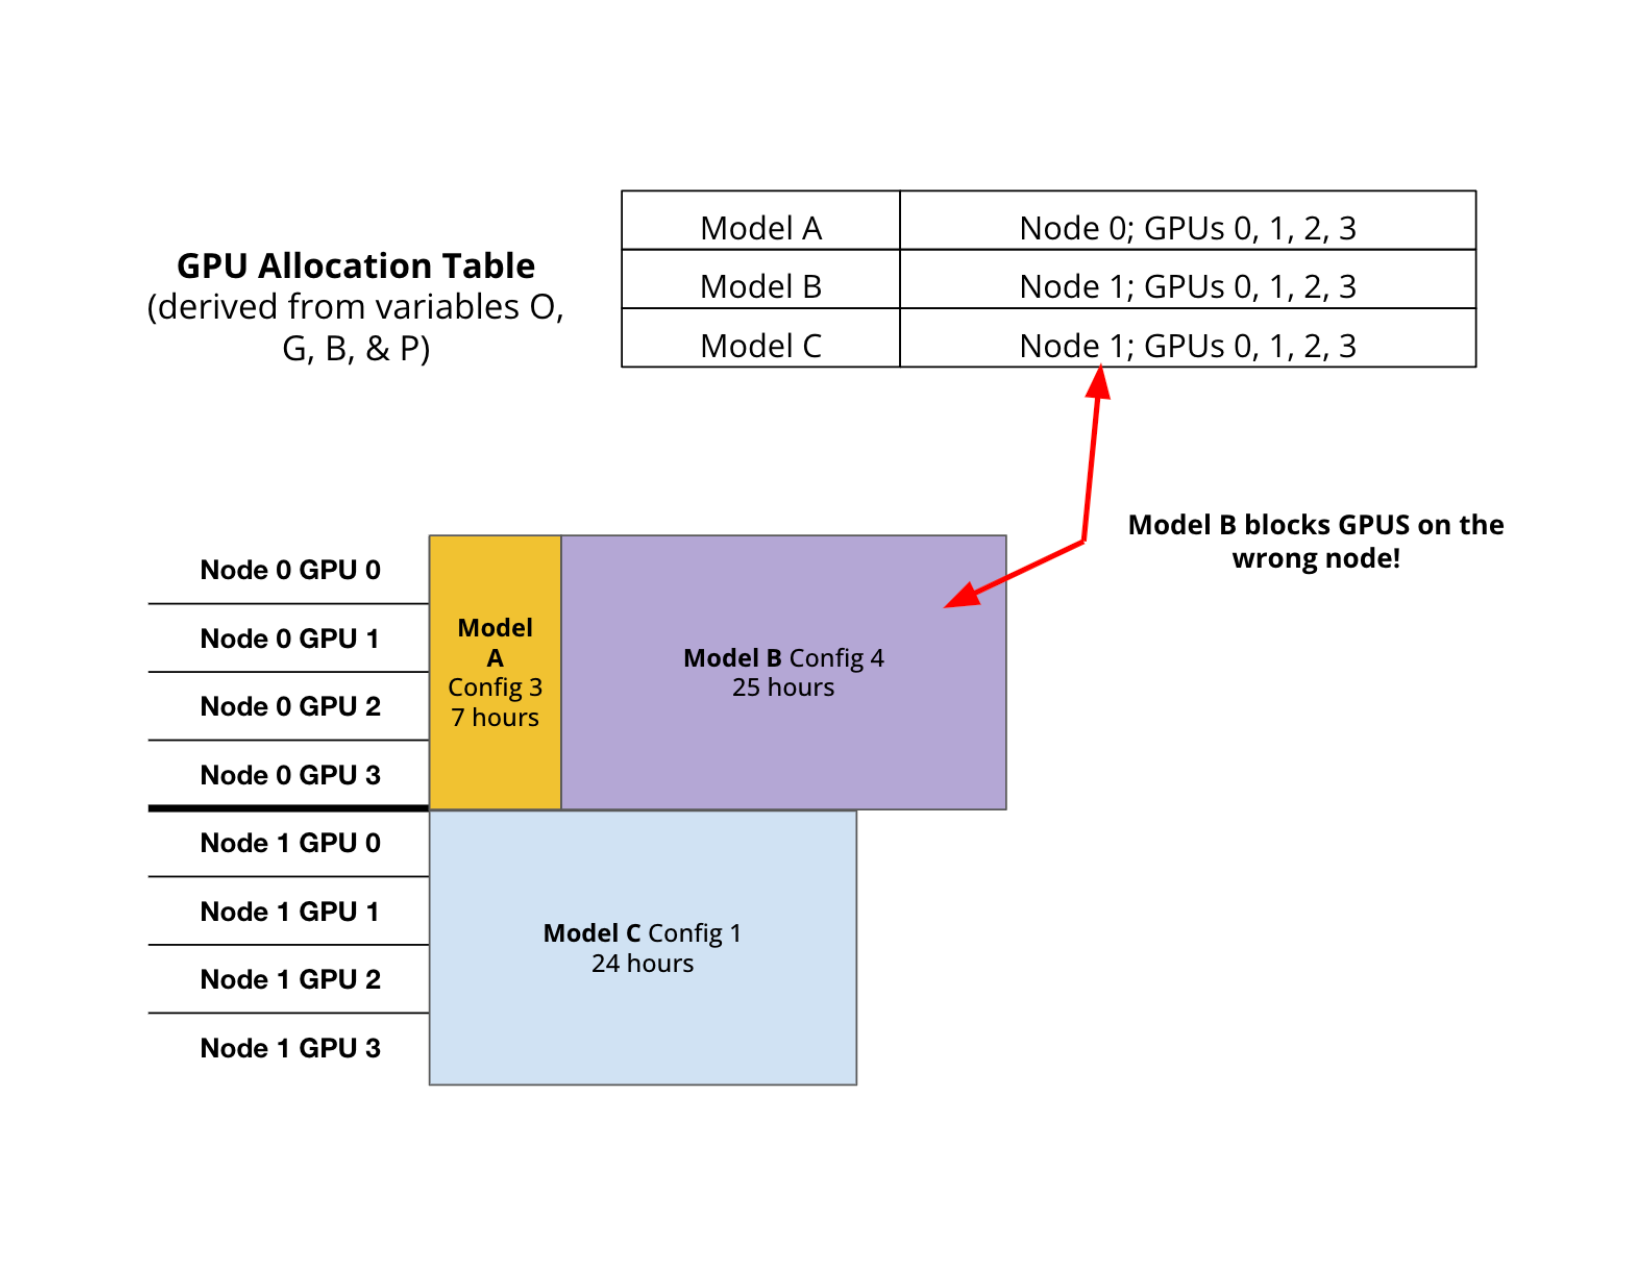}
\vspace{-3mm}
\caption{Illustration of a \spase~solution where a task blocks GPUs on a node it has not selected, violating constraints 6 \& 7.}
\label{fig:milp_illustration_constraint6}
\end{figure}

\vspace{2mm}

\textbf{Constraints 8 and 9.}

Constraints 8 \& 9 enforce gang scheduling semantics, so that if a job is assigned multiple GPUs, it will start executing on all GPUs simultaneously. 

\vspace{-2mm}	
\begin{align}
\tag{\ref{eqn:gpu_gang_a}}
\begin{split}
\frac{\sum_{x \in I_{t,n}} x}{G_{t, s}} \leq I_{t,n,g} + U \times (3 - P_{t,n,g} - B_{t,s}  - O_{t,n}) \\ \forall s \in S_{t}, \forall t \in T, \forall g \in GPU_{n}, \forall n \in N
\end{split}
\end{align}

\begin{align}
\tag{\ref{eqn:gpu_gang_b}}
\begin{split}
\frac{\sum_{x \in I_{t,n}} x}{G_{t, s}} \geq I_{t,n,g} - U \times (3 - P_{t,n,g} - B_{t,s}  - O_{t,n}) \\ \forall s \in S_{t}, \forall t \in T, \forall g \in GPU_{n}, \forall n \in N
\end{split}
\end{align}

\begin{figure}[H]
\includegraphics[width=0.95\columnwidth]{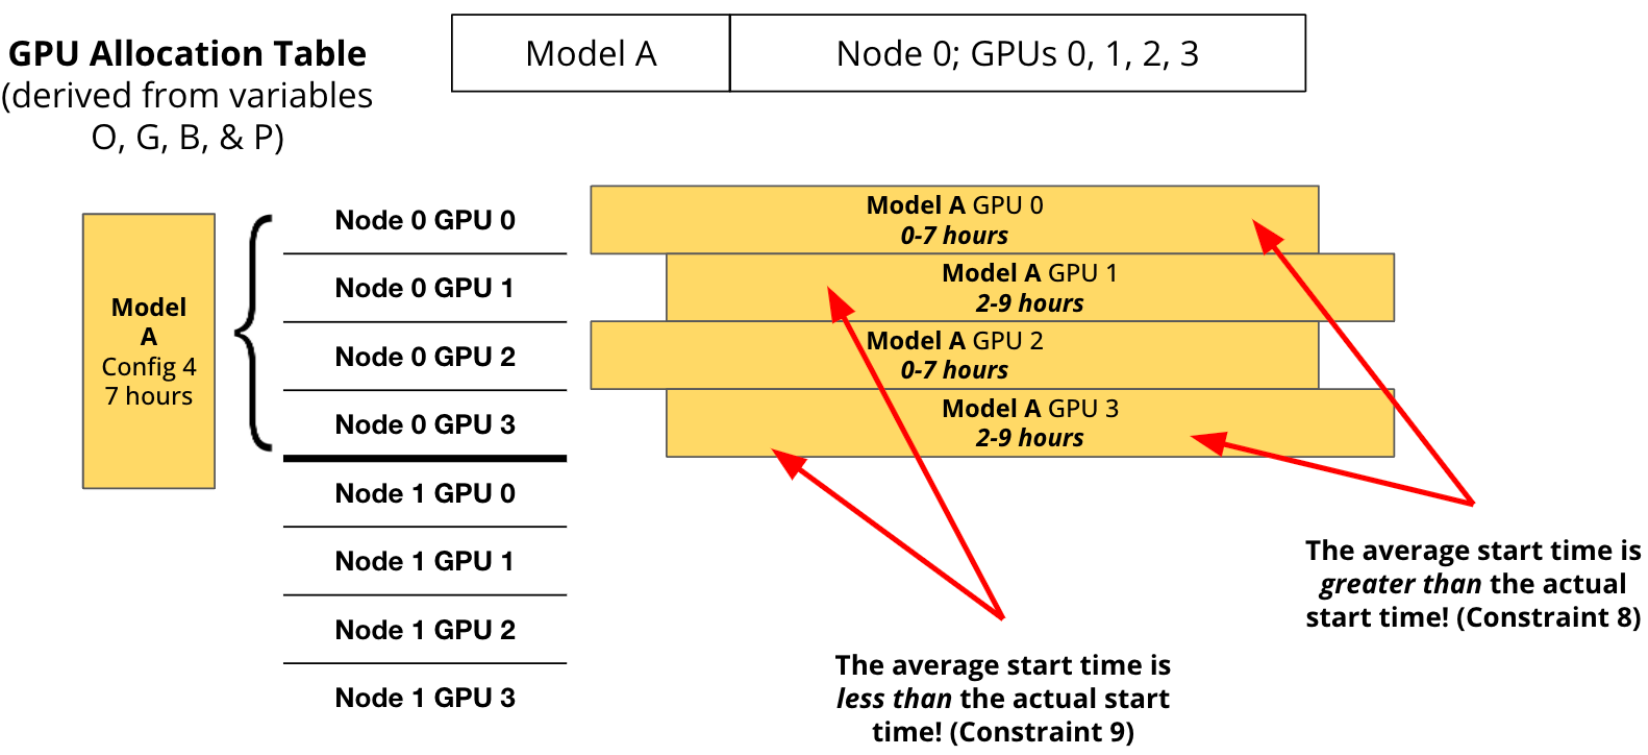}
\vspace{-3mm}
\caption{Illustration of a specific model violating gang scheduling requirements, thus breaking Constraints 8 \& 9.}
\label{fig:milp_illustration_constraint8}
\end{figure}

\vspace{2mm}

\textbf{Constraints 10 and 11.}

Finally, Constraints 10 and 11 ensure that if two jobs share any GPUs in common, then their active runtimes cannot overlap.

\begin{align}
\tag{\ref{eqn:task_isolation_a}}
\begin{split}
I_{t1,n,g} \leq I_{t2,n,g} - R_{t,s} + U \times ((3 - P_{t1,n,g} - P_{t2,n,g}) - B_{t,s} + A _{t2, t1}) \\ \forall s \in S_{t}, \forall t1 \in T, \forall t2 \in (T - \{t1\}), \forall g \in GPU_{n}, \forall n \in N
\end{split}
\end{align}

\begin{align}
\tag{\ref{eqn:task_isolation_b}}
\begin{split}
I_{t1,n,g} \geq I_{t2,n,g} + R_{t,s} - U \times ((4 - P_{t1,n,g} - P_{t2,n,g}) - A _{t2, t1} - B_{t,s}) \\ \forall s \in S_{t}, \forall t1 \in T, \forall t2 \in (T - \{t1\}), \forall g \in GPU_{n}, \forall n \in N
\end{split}
\end{align}

\begin{figure}[H]
\includegraphics[width=0.95\columnwidth]{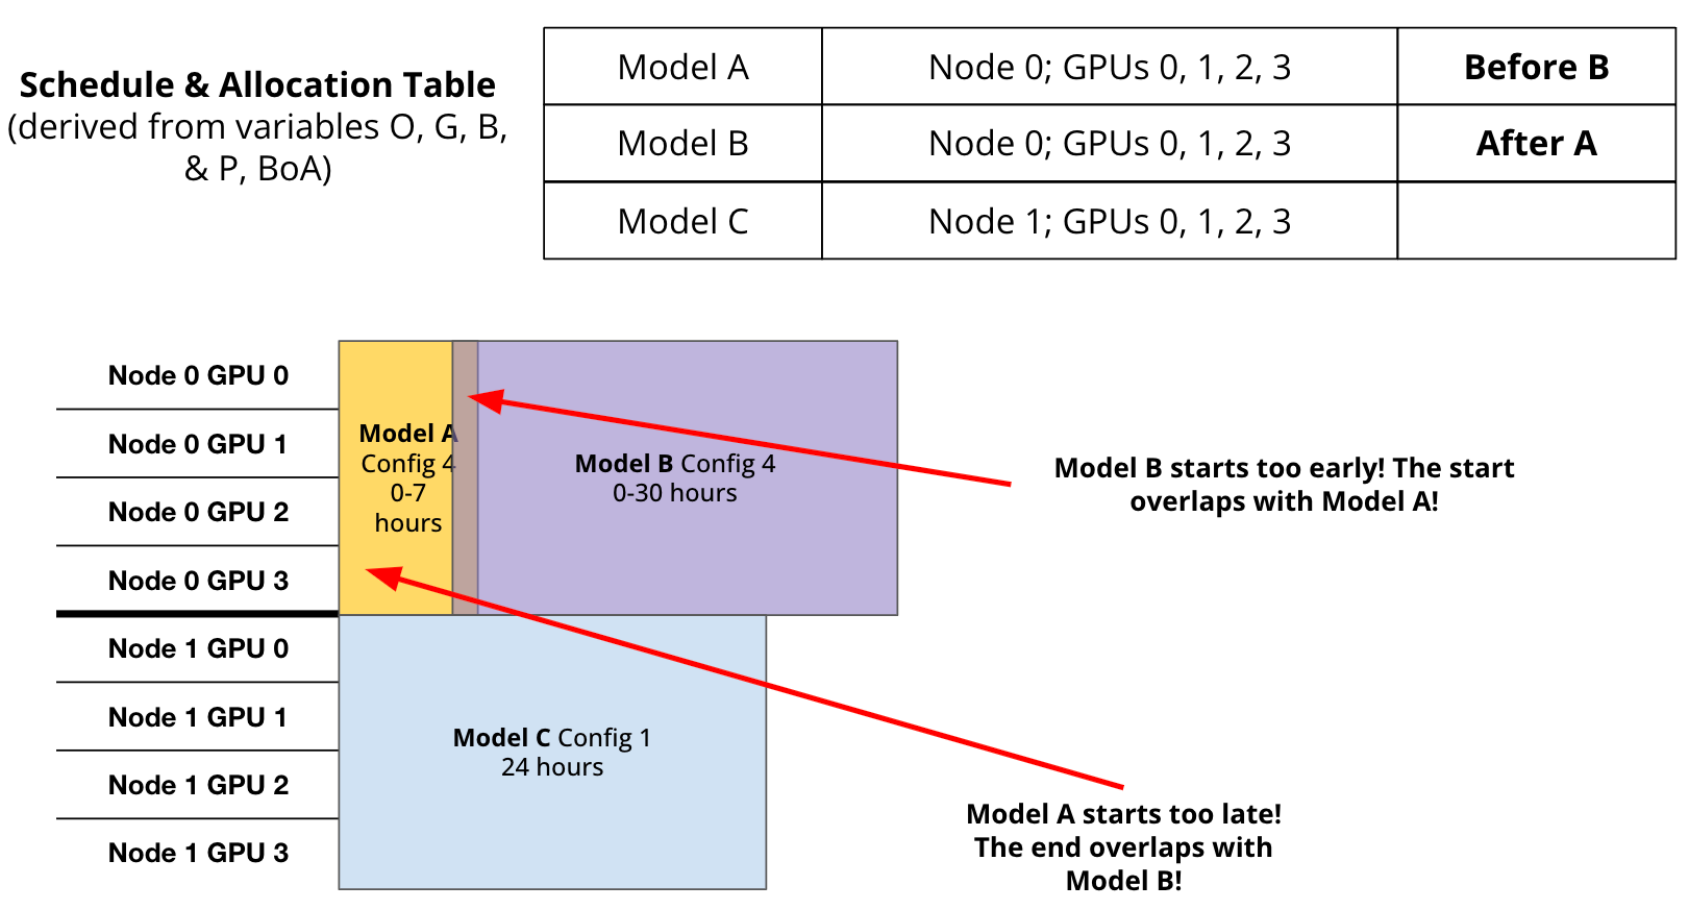}
\vspace{-3mm}
\caption{Illustration of a \spase~execution plan violating task isolation requirements, thus breaking Constraints 10 \& 11.}
\label{fig:milp_illustration_constraint8}
\end{figure}

\section{Interval Introspection}
Here, we provide the basic algorithm for our introspective solver.
Essentially, we re-trigger the solver on a fixed interval and determine if the new solution improves performance versus just continuing with the existing plan.
If the new plan is superior, we checkpoint all active jobs and re-launch with the new plan.

\begin{algorithm}[h]
\caption{:~\textsc{\textbf{Round Introspection}}(Workload $W$, Interval $I$)}
\label{alg:dynamic_rescaler}
\begin{algorithmic}[1]
\STATE $\text{Schedule} S = MILP(W)$
\STATE $M = Makespan(S)$
\STATE $\text{E2ESchedule} = S[0:I]$
\STATE $\text{T} = 500$
\WHILE{\text{W not exhausted}}
	\STATE $W = W \text{ after } I \text{ seconds of } S$
	\STATE $S = S[I:]$
	\STATE $M = M - I$
	\STATE $\text{Proposal} = MILP(W)$
	\IF  {\text{Makespan(Proposal)} $\leq$ M - T }
		\STATE $S = \text{Proposal}$
		\STATE $M = \text{Makespan(Proposal)}$
	\ENDIF
	\STATE $E2ESchedule.append(S[0:I])$
\ENDWHILE
\RETURN $L$
\end{algorithmic}
\end{algorithm}

We use a tolerance level, $T$, to describe the minimum acceptable benefit of an introspective plan switch.
If the swap only provided a 5 second benefit, for example, the switching overheads alone might outweigh the makespan reduction.

\section{Additional Related Works}
In this section, we go into some other DL systems works that are relevant to performance optimization in general, though they do not overlap directly with the specifics of our \spase~problem.

\vspace{2mm}
\noindent \textbf{Pipelining \& FSDP:} 
Pipelining is a modification of model parallelism in which the model is sharded in a sequential fashion. 
It partitions a minibatch into smaller ``microbatches,'' then shuttles the microbatches through the model partitions~\cite{yang2020pipemare,gpipe2018,torchgpipe2020,terapipe2021}.
This enables different model shards to concurrently run different microbatches. 
%Pipelining generally suffers from \textit{synchronization} overheads between prediction and backpropagation steps.
%Some asynchronous schemes exist to mitigate this issue, but they affect execution correctness.
The speedup of pipelining is heavily tied to the partitioning scheme and the number of microbatches.
Prior work has underscored the importance of tuning these knobs via either expert knowledge or automated heuristics~\cite{terapipe2021}.

Fully-Sharded-Data-Parallelism (FSDP) is a more recent approach that blends model parallelism with data parallelism. Originally introduced in Microsoft's ZeRO~\cite{zero2019}, it has since been integrated into the PyTorch Distributed package~\cite{torchddp2020}. 
FSDP partitions a model graph across multiple accelerators, then sends different minibatch partitions to the accelerators. FSDP runs All-Gather on model layers in sequence as data moves through the graph. 
The currently executing layer group is data-parallel-replicated; the other operators are still distributed in a model-parallel way. 
%This allows users to benefit from both data parallel processing and model parallel memory distribution.
FSDP exposes two main user-configured optimizations to reduce GPU memory pressure: (1) gradient checkpointing~\cite{checkpointing2016} and (2) DRAM spilling. 
%Checkpointing applies a popular memory reduction technique on top of the layer partitioning. 
%Offloading borrows from spilling (described below) to push some layers to main system memory when they are not executing. 
Turning these knobs on can lower GPU memory pressure at the cost of some performance. 
Ascertaining when it is worth turning one or both of these techniques generally requires empirical testing.    

\vspace{2mm}
\noindent \textbf{DL Cluster Schedulers:} 
Schedulers such as Gandiva, Apollo, Tiresias, \& Antman target a different setting~\cite{xiao2020antman,xiao2018gandiva,boutin2014apollo,gu2019tiresias,bao2019deep} and require manual resource specification. Gandiva does offer opportunistic rescaling for elastic~\cite{wu2019elastic} jobs, but without knowledge of the model's scalability. These systems and other orchestrators like Pathways~\cite{pathways2022} tackle systems challenges that arise with very large clusters. 
Our focus is \textit{complementary} in that we aim to free end users of DL from needing to hand-tune systems factors. 
%They consider problems such as colocation, GPU-sharing (for small models), memory rescaling within an accelerator, and heterogeneous resource management. 
One could potentially integrate \system~with such larger schedulers by allocating a set of nodes for \system~to manage locally for model selection.
Gavel~\cite{gavel2020} schedules over heterogeneous resources, which is beyond our scope, but does not tackle the \spase~problem. Their metrics to handle heterogeneity could potentially be used in a future \system~extension.

\vspace{2mm}
\noindent \textbf{System Optimizers:} KungFu~\cite{maikungfu2020} provides an interface for users to express various procedures for mid-training system parameter changes.
Litz~\cite{litz2018} provides a programming model for elastic parameter server data parallelism.
TeraPipe uses dynamic programming to optimize the partitioning and execution of pipeline parallelism~\cite{terapipe2021}.
Systems like Rammer~\cite{rammer2020}, GO~\cite{GO}, TVM~\cite{tvm}, SystemML's query rewriter~\cite{fusion2018} and compiler autotuners~\cite{autotuning,agnostic2018} provide similar up-front optimizations for DL workloads.
These automated search procedures are orthogonal to our own work and support can be added in the future using our UPP abstraction and Library API.

\vspace{2mm}
\noindent \textbf{Other Model Selection Systems:} Nautilus~\cite{nakandala2022nautilus} optimizes model selection for transfer learning. $\alpha$-NAS~\cite{alphaNas2022} proposes a method for creating architecture search workloads.
Other systems like FairRover~\cite{fairness2021} tackle human-in-the-loop model building.
These works are orthogonal to our own --- they create/modify the model selection workload that \system~executes.

\vspace{2mm}
\noindent \textbf{Other DL System Optimizations:} Optimizations such as compilation~\cite{tvm,tf-xla,tflms2019,compiler,autotuning}, batching~\cite{hivemind, retiarii, packed-models}, compression~\cite{compression,distilling,scma2021}, and graph substitution~\cite{taso2019,metaflow2019,unger2022unity} are orthogonal to our work. Many systems (e.g. DeepSpeed~\cite{zero2019,zero2021,zerooffload2021}, Megatron~\cite{megatronlmgpuscaling2021,megatron2019,megatronlmblog2020}, Hotline~\cite{hotline2022}, HugeCTR~\cite{hugeCTR}, RecShard~\cite{dlrm2019,dlrmscale2020}, HogBatch~\cite{9460628}, and Switch Transformers~\cite{fedus2021switch})  propose new parallelisms, all expressible under our Library API.
Data pipeline optimizations~\cite{redyuk2022dorian,wang2021gradient,wang2018dataset,datacol2021}, fairness systems~\cite{omnifair2021,mlinspect2021,fairsample2021}, and end-to-end pipeline managers~\cite{systemds2019,baylor2017tfx,keystone2016,lima2021,petuum2015} are also mostly orthogonal to our own work; we do not restrict the workload/data design. Some other works have addressed large-model challenges in different ways; e.g. by using alternative, parameter-efficient architectures~\cite{param2021} or else by training on non-GPU hardware~\cite{slide2021,sun2021deep}. By contrast, \system~is intended to optimize existing large-model GPU-training settings.
Still other works optimize for settings such as DL inference~\cite{9203676,8486422,nakandala2020incremental,videoanalytics,figo,thia2021} or non-DL compute~\cite{grandl2014multi-resource,yarn2013,mesos2011,halideSearch2019,vahid2014,slaq2017}. These works target a different setting entirely.
%----------------------------------------------------------------------------------------------------------------
